# Supplementary material for: Unreliable Partial Label Learning with Recursive Separation
Source: arXiv:2302.09891 source file (2023-08-29)
Supplement: Supplementary file 1 [file Appendix.tex]

\section{Appendix}

\subsection{Label Updating for Augmented Solution}
Analogous to the General Solution, $\mathrm{w}_{ij}$ represents the confidence that the $j$-th class is the true label for the $i$-th instance. 
For an instance $i$, if the $j$-th class is not included in the candidate label set, then $\mathrm{w}_{ij}=0$, otherwise, $\mathrm{w}_{ij}$ takes the form as follows:
\begin{equation}
    \mathrm{w}_{ij}=\frac{\left(\prod_{\boldsymbol{z} \in \mathcal{A}(\boldsymbol{x}_{i})} g_j(\boldsymbol{z})\right)^{\frac{1}{|\mathcal{A}(\boldsymbol{x})|}}}{\sum_{k \in s_i}\left(\prod_{\boldsymbol{z} \in \mathcal{A}(\boldsymbol{x}_{i})} g_k(\boldsymbol{z})\right)^{\frac{1}{|\mathcal{A}(\boldsymbol{x})|}}},
    \label{CR}
\end{equation}
where $g_j(\cdot)$ is the $j$-th coordinate of $g(\cdot)$. For initialization, the weights are uniform, i.e.
\begin{equation}
    \mathrm{w}_{ij}=\left\{\begin{array}{cl}
    \frac{1}{|s_{i}|} & \text { if } j \in s_{i}, \\
    0 & \text { otherwise. }
    \end{array}\right.
\end{equation}

\begin{algorithm}[tb]
    \caption{UPLLRS Algorithm with Augmented Solution}
    \label{alg:UPLLRS+}
    \textbf{Input}: Network $g(\cdot; \omega)$ with parameters $\omega$.
    Unreliable partial label dataset $\tilde{D}$ and validation set $V$. 
    Max training epochs $T$.   \\
    \textbf{Output}: Parameters $\omega$ for $g(\cdot)$.

    \begin{algorithmic}[1] %[1] enables line numbers.
    \STATE Obtain reliable subset $\tilde{D}_{R}^{\lambda}$ and 
    unreliable partial dataset $\tilde{D}_{U}^{\lambda}$ by employing Algorithm \ref{alg:RS} in main body;
    \STATE Randomly initialize $\omega$.
    \FOR{$i \leftarrow 1$ to $T$}
        \STATE Train $g(\cdot;\omega)$ from $\tilde{D}_{R}^{\lambda}$;
        \STATE Calculate loss according Eq. \ref{Eq.loss} in main body;
        \STATE Update labels according Eq. \ref{CR};
    \ENDFOR
    \STATE \textbf{return} $\omega$.

    \end{algorithmic}
\end{algorithm}
\subsection{Experiment Details}

\subsubsection{Datasets}
\begin{itemize}
    \item CIFAR-10 contains 60,000 (50,000 in the training set and 10, 000 in the test set) $32 \times 32 \times 3$ RGB images including 10 classes: airplane, bird, automobile, cat, deer, frog, dog, horse, ship, and truck. Each class has 5000 training images and 1000 test images.
    \item CIFAR-100 contains 60,000 (50,000 in the training set and 10, 000 in the test set) $32 \times 32 \times 3$ RGB images including 100 classes. Each class has 500 training images and 100 test images.
    \item Dermatology contains 34 attributes, 33 of which are linear valued and one of them is nominal. The objective of this dataset is to determine the type of Eryhemato-Squamous Disease. The dataset comprises of 366 instances.
    \item 20Newsgroups dataset comprises of 20,000 instances and is characterized as a text dataset. In accordance with prior research of PLL, it is widespread practice to preprocess text data by converting it into feature vectors of double type, with a size of 300.
\end{itemize}

It is more equitable to report the test accuracy when the accuracy on the validation set reaches its peak.
Given that the aforementioned datasets do not include a validation set, in order to promote a more equitable comparison, we partition the aforementioned four datasets into training, validation, and test sets in a 4:1:1 ratio.
For example, the CIFAR-10 and CIFAR-100 synthesized datasets both have 40, 000 training images, 10, 000 validation images and 10, 000 test images. 

The data augmentation techniques used for CIFAR-10, CIFAR-100 are: (1) Random Horizontal Flipping, (2) Random Cropping, (3) Cutout, and (4) Auto Augment.
It should be noted that the evaluation of the partial label learning methods, PiCO and CR-DPLL, was not conducted on the Dermatology and 20Newsgroups.
Given that both methods utilize image argumentation as a crucial component, they are specifically tailored for image datasets and are not applicable to the Dermatology or the 20Newsgroups dataset.
Specifically, the utilization of contrastive learning in PiCO enables the effective representation of features through the incorporation of an augmented perspective of an image, facilitating the computation of similarity scores.
CR-DPLL employed consistency regularization through the utilization of data augmentation in three different ways.

\subsection{Supplementary Ablation Study}

\subsubsection{Analysis of Parameter $\xi$}

\begin{table}[t]
    \centering
    \resizebox{0.99\columnwidth}{!}{
        % Table generated by Excel2LaTeX from sheet 'Ablation'
        \begin{tabular}{c|c|c|c}
            \toprule
                & $\xi$ & $\mu=0.3$ & $\mu=0.5$ \\
            \midrule
            \multirow{3}[2]{*}{CIFAR-10 ($\eta=0.3$)} & 0.5   & 92.80 $\pm$ 0.39\% & 90.30 $\pm$ 0.54\% \\
                & 1     & 93.37 $\pm$ 0.31\% & 90.92 $\pm$ 0.79\% \\
                & 2     & \textbf{93.85} $\pm$ 0.31\% & \textbf{91.16} $\pm$ 0.67\% \\
            \midrule
            \multirow{3}[2]{*}{CIFAR-100 ($\eta=0.05$)} & 0.3   & 70.31 $\pm$ 0.22\% & \textbf{64.78} $\pm$ 0.53\% \\
                & 0.5   & \textbf{70.46} $\pm$ 0.65\% & 64.52 $\pm$ 0.51\% \\
                & 1     & 69.84 $\pm$ 0.41\% & 64.35 $\pm$ 0.58\% \\
            \bottomrule
            \bottomrule
            \end{tabular}%
    }
    \caption{The impact of varying values of $\xi$ on the accuracy (mean $\pm$ std).}
    \label{tab:xi}
\end{table}

In order to evaluate the impact of the scalar hyperparameter $\xi$, we conduct a performance comparison analysis.
All other parameters are maintained at their initial values as established in the primary experiment.
As shown in Table \ref{tab:xi}, we investigate the impact of varying the parameter $\xi$ on the performance of our proposed algorithm.
Specifically, on the CIFAR-10 dataset, we consider three values of $\xi$: 0.5, 1, and 2. 
As for CIFAR-100 dataset, we consider three values of $\xi$: 0.3, 0.5, and 1. 
Our findings demonstrate that, when evaluating on the CIFAR-10 dataset, an increase in $\xi$ corresponds to an improvement in the performance. 
Conversely, on the CIFAR-100 dataset, an increase in $\xi$ results in a decline in the performance of the proposed method.
Based on the results of our ablation study, we empirically determined that the value of $\xi$ for the CIFAR-10 dataset is 2, while for the CIFAR-100 dataset, the value of $\xi$ is 0.3 in our experiment.

\subsubsection{Analysis on $\gamma$ (Seperation Rate)}

\begin{table}[t]
    \centering
    \resizebox{0.99\columnwidth}{!}{
        % Table generated by Excel2LaTeX from sheet 'Ablation'
        \begin{tabular}{c|c|c|c}
            \toprule
                & $\gamma$ & $\mu=0.3$ & $\mu=0.5$ \\
            \midrule
            \multirow{4}[2]{*}{CIFAR-10 ($\eta=0.3$)} & 0.005  & 92.32  $\pm$ 0.81\% & 90.78  $\pm$ 0.25\% \\
                & 0.01  & 92.94  $\pm$ 0.06\% & 90.83  $\pm$ 0.11\% \\
                & 0.03  & \textbf{93.37} $\pm$ 0.31\% & 90.92 $\pm$ 0.79\% \\
                & 0.05  & 93.06  $\pm$ 0.37\% & \textbf{91.90}  $\pm$ 0.44\% \\
            \midrule
            \multirow{4}[2]{*}{CIFAR-100 ($\eta=0.05$)} & 0.005 & 69.84  $\pm$ 0.41\% & \textbf{64.35}  $\pm$ 0.58\% \\
                & 0.01  & \textbf{70.81}  $\pm$ 0.48\% & 64.11  $\pm$ 0.58\% \\
                & 0.03  & 69.01  $\pm$ 0.70\% & 61.76  $\pm$ 0.46\% \\
                & 0.05  & 66.57  $\pm$ 0.76\% & 59.46  $\pm$ 1.06\% \\
            \bottomrule
            \bottomrule
            \end{tabular}%
    }
    \caption{The impact of varying values of $\gamma$ on the accuracy (mean $\pm$ std).}
    \label{tab:gamma}
\end{table}

To assess the effect of the scalar hyperparameter $\gamma$ on the performance, we conduct a comparative analysis.
In these supplementary experiments, all parameters were held constant at their values established in the primary experiment, with the exception of the scalar hyperparameter $\xi$, which was set to a value of 1.
In our experiments, we test a range of values for the scalar hyperparameter $\gamma$, specifically, we test $\gamma$ values in the set $\{0.005, 0.01, 0.03, 0.05\}$.
Our results in Table \ref{tab:gamma} indicate that the self-adaptive strategy employed in our method limits the impact of the separation rate $\gamma$, as it is designed to terminate at an appropriate time.
Although the impact of separation rate is limited, our ablation results reveal that the proposed method demonstrates improved performance when $\gamma$ is set to 0.03 or 0.05 on the CIFAR-10 dataset, and to 0.005 or 0.01 on the CIFAR-100 dataset. These results suggest that, for optimal performance on the CIFAR-10 dataset, a larger value of $\gamma$ is preferable, while a smaller value is preferable for the CIFAR-100 dataset.
In general, a larger value of the scalar hyperparameter $\gamma$ corresponds to a more aggressive strategy, which may result in a greater number of correct samples added to the unreliable subset and a smaller reliable subset. 
One potential explanation for this is that the CIFAR-10 dataset, which contains a larger number of samples per class, allows for more robust representation learning due to the presence of a greater number of reliable samples.
Empirically, through our experiments, we have determined that an optimal value of the scalar hyperparameter $\gamma$ for the CIFAR-10 dataset is 0.03 and for the CIFAR-100 dataset is 0.005.

\subsection{Computational Efficiency}
The stage 1 of UPLLRS takes approximately 60 seconds per exclusion step (0.28M parameters), which includes 5-epoch training and sorting. Stage 2 requires approximately 2m per epoch (1.47M parameters) with batch size of 256. For instance, on the CIFAR-10 dataset with $\eta=0.5, \mu=0.3$ and seed 0 (RTX3090), the total cost for stage 1 is approximately 12m (14 exclusion steps). In the
stage 2, the total epoch is 263 stopped by early-stopping, cost
8h 29m 42s.
